# Supplementary material for: Revisiting the Effects of Stochasticity for Hamiltonian Samplers
Source: arXiv:2106.16200 source file (2021-11-04)
Supplement: Supplementary file 1 [file sectionleapappendix.tex]

\subsection{Analytical solution of Ornstein-Uhlenbeck process}\label{sec:ouanalytic}
We here derive the analytical solution of an Ornstein-Uhlenbeck process for the analytical steps of certain numerical schemes.
The process under study has the following form 
\begin{equation}
    \mathbf{dr}(t)=-C\mathbf{M}^{-1}\rvect(t)dt-\mathbf{f}dt+\sqrt{2C}\mathbf{dw}(t)
\end{equation}
that can be rewritten, with $\boldsymbol{\mu}=(C\mathbf{M}^{-1})^{-1}\mathbf{f}$, as

\begin{equation}
    \mathbf{dr}(t)=-C\mathbf{M}^{-1}(\rvect(t)-\boldsymbol{\mu})dt+\sqrt{2C\eye}\mathbf{dw}(t)
\end{equation}
that has analytic solution
\begin{equation}\label{ousol}
    \rvect(t)=\exp(-C\mathbf{M}^{-1}t)(\rvect(0)-\boldsymbol{\mu})+\boldsymbol{\mu}+\sqrt{2C}\int\limits_{0}^{t} \exp(-C\mathbf{M}^{-1}(t-s))\mathbf{dw}(s)
\end{equation}
By taking the differential of \cref{ousol} indeed
\begin{flalign*}
& \mathbf{dr}(t)=-C\mathbf{M}^{-1}\exp(-C\mathbf{M}^{-1}t)(\rvect(0)-\boldsymbol{\mu})+
\sqrt{2C}\exp(-C\mathbf{M}^{-1}(t-t))\mathbf{dw}(t)\\&-C\mathbf{M}^{-1}\sqrt{2C}\int\limits_{0}^{t} \exp(-C\mathbf{M}^{-1}(t-s))\mathbf{dw}(s)\\&=-C\mathbf{M}^{-1}\left(\exp(-C\mathbf{M}^{-1}t)(\rvect(0)-\boldsymbol{\mu})+\sqrt{2C}\int\limits_{0}^{t} \exp(-C\mathbf{M}^{-1}(t-s))\mathbf{dw}(s)\right)+
\sqrt{2C}\mathbf{dw}(t)=\\
&-C\mathbf{M}^{-1}\left(\rvect(t)-\boldsymbol{\mu}\right)dt+
\sqrt{2C}\mathbf{dw}(t).
\end{flalign*}
The $\boldsymbol{\mu}$ term in the solution is added to ensure the consistency with initial conditions, 
\begin{equation}
\rvect(0)=(\rvect(0)-\boldsymbol{\mu})+\boldsymbol{\mu}+\zerovect=\rvect(0)
\end{equation}
To derive the ``algorithmic'' version it is necessary to compute the variance of the noise term at a given time instant
\begin{flalign*}
&\sqrt{2C}\int\limits_{0}^{t} \exp(-C\mathbf{M}^{-1}(t-s))\mathbf{dw}(s)\sqrt{2C}\int\limits_{0}^{t} \exp(-C\mathbf{M}^{-1}(t-q))\mathbf{dw}(q)=\\
&2C\int\limits_{0}^{t} \exp(-2C\mathbf{M}^{-1}(t-s))ds=2C\exp(-2C\mathbf{M}^{-1}t)\int\limits_{0}^{t} \exp(2C\mathbf{M}^{-1}s)ds=\\
&2C\exp(-2C\mathbf{M}^{-1}t)\left(\exp(2C\mathbf{M}^{-1}t)-\eye\right)(2C\mathbf{M}^{-1})^{-1}=\mathbf{M}(\eye-\exp(-2C\mathbf{M}^{-1}t)),
\end{flalign*}
providing an equivalent representation 
\begin{equation}\label{ousolN}
    \rvect(t)=\exp(-C\mathbf{M}^{-1}t)(\rvect(0)-\boldsymbol{\mu})+\boldsymbol{\mu}+\sqrt{\mathbf{M}(1-\exp(-2C\mathbf{M}^{-1}t))}\mathbf{w},\quad \mathbf{w}\sim \mathcal{N}(\zerovect,\eye).
\end{equation}
When $\mathbf{M}$ is diagonal, the exponential matrix is diagonal with entries obtained by exponentiating its diagonal elements.
%% Whenever the matrix $\mathbf{M}$ is diagonal, the exponential matrix is just the entrywise exponential.

The Stochastic Position verlet scheme (order-two, the "correct" leapfrog) can then be derived as
\begin{equation}\label{eq:spv}
    \begin{cases}
    \thetavect^*=\thetavect_0+\frac{\eta}{2}\mathbf{M}^{-1}\rvect_0\\
    \rvect_1=\exp(-C\mathbf{M}^{-1}\eta)\rvect_0+\left(\eye-\exp(-C\mathbf{M}^{-1}\eta)\right)\frac{\mathbf{M}}{C}\nabla U(\thetavect^*)+\sqrt{\mathbf{M}(1-\exp(-2C\mathbf{M}^{-1}\eta))}\mathbf{w}\\
    \thetavect_1=\thetavect^*+\frac{\eta}{2}\mathbf{M}^{-1}\rvect_1.\\
    \end{cases}
\end{equation}

\subsection{Detailed \leapfrog analysis}\label{sec:leapmir}
The purpose of this section is to explore in detail the mathematical properties of the \leapfrog scheme, the most commonly adopted numerical integrator in the Bayesian sampling community.

The deterministic \leapfrog is a known deterministic integrator. When considering \sdes, it is possible to derive its stochastic counterpart as a blind generalization of the deterministic leapfrog scheme, i.e. starting from
\begin{equation}\label{eq:detleap}
    \begin{cases}
    \thetavect^*=\thetavect_0+\frac{\eta}{2}\mathbf{M}^{-1}\rvect_0\\
    \rvect_1=\rvect_0-\eta \nabla U(\thetavect^*)\\
    \thetavect_1=\thetavect^*+\frac{\eta}{2}\mathbf{M}^{-1}\rvect_1\\
    \end{cases}
\end{equation}
the following scheme is constructed
\begin{equation}\label{eq:stoleap3}
    \begin{cases}
    \thetavect^*=\thetavect_0+\frac{\eta}{2}\mathbf{M}^{-1}\rvect_0\\
    \rvect_1=\rvect_0-\eta \nabla U(\thetavect^*)-\eta C \rvect_0+\sqrt{2 C\eta}\mathbf{w},\quad \mathbf{w}\sim \mathcal{N}(\zerovect,\eye)\\
    \thetavect_1=\thetavect^*+\frac{\eta}{2}\mathbf{M}^{-1}\rvect_1.\\
    \end{cases}
\end{equation}
Notice that in practical implementations the first and last step are merged into a single step with the exception of the beginning and end of the chain. This does not pose a problem in that usually we are intrested only in functions of the position.

Importantly, the deterministic \leapfrog is order-two. The steps of the scheme \cref{eq:detleap} are analytic solutions of differential equations, and the integration induces operators
\begin{equation}
  \exp\left(\frac{\eta}{2}\left(\nabla^\top_{\rvect}T(\rvect)\right)\nabla_{\thetavect}\right)\exp\left(-\eta\left(\nabla^\top_{\thetavect}U(\thetavect)\right)\nabla_{\rvect}\right)\exp\left(\frac{\eta}{2}\left(\nabla^\top_{\rvect}T(\rvect)\right)\nabla_{\thetavect}\right)=\exp\left(\eta\mathcal{H}\right)+\mathcal{O}(\eta^3).
\end{equation}
The result is immediate remembering that $\mathcal{H}=-\left(\nabla^\top_{\thetavect}U(\thetavect)\right)\nabla_{\rvect}+\left(\nabla^\top_{\rvect}T(\rvect)\right)\nabla_{\thetavect}$ and using the BCH formula \cref{secproof:bch}.

The stochastic \leapfrog, \cref{eq:stoleap3}, instead, is order-one. While the position update steps are analytic, the momentum update \begin{equation}\label{eumom}
    \rvect_1=\rvect_0-\eta \nabla U(\thetavect^*)-\eta C \rvect_0+\sqrt{2 C\eta}\mathbf{w}
\end{equation} is not anymore an analytic step but it is an \euler step, thus with an error $\mathcal{O}(\eta^2)$. Consequently, the scheme of \cref{eq:stoleap3} induces an operator as follows
\begin{equation}
    \exp(\frac{\eta}{2}\mathcal{D})\left(\exp\left(\eta\mathcal{H}\right)+\mathcal{O}(\eta^2)\right)\exp(\frac{\eta}{2}\mathcal{D})=\exp\left(\eta\mathcal{L}\right)+\mathcal{O}(\eta^{\min(2,3)})=\exp\left(\eta\mathcal{L}\right)+\mathcal{O}(\eta^{2}).%+\mathcal{O}(\eta^2)+\mathcal{O}(\eta^3)
\end{equation}

Despite being formally order-one, we found no empirical difference between the stochastic \leapfrog scheme and other quasi-symplectic order-two schemes. Similar results have been observed in the \sde simulation literature, look for example at \cite{milstein2003quasi}, Table 1. The possible explanation is that while the stochastic \leapfrog is not order-two, it is nevertheless a quasi symplectic scheme. This important geometrical property can explain the robustness of the scheme. 

Here we explore the differential operator $\mathcal{U}, \mathbb{E}[\phi(\zvect_{\mathbf{1}})|\zvect_{\mathbf{0}}] = \mathcal{U}\phi$ explicitly, by expanding it in Taylor series and comparing it with the expansion of the true operator $\exp(\eta\mathcal{L})$.
As expected, we explicitly prove that the integrator is at least order-one.

We consider the Taylor expansion of the operator $\mathcal{U}$ induced by the numerical scheme and focus on the $\eta^2$ terms. To be exactly of order two, we would need the combination of such terms to be equal to $\mathcal{L}^2$. To check whether this holds or not, we compare the expansion of $\mathcal{U}$, \cref{expu}, and the operator $\mathcal{L}^2$, \cref{expl}, and verify indeed that there is not a matching, according to the statement that \leapfrog is order one. We believe however that the explanation of the performance of \leapfrog scheme, on par with other second order schemes, can be understood by considering that many of the summands of \cref{expu},\cref{expl} coincide and that the scheme is quasi-symplectic. Our is however an educated guess at best, and not a mathematical proof. The interested reader could use our discussion as a starting point for a precise analysis.

For simplicity, we expose our reasoning for the one-dimensional case.
We define $f=\frac{\partial U}{\partial \theta}$, and we start by manipulating the expression for the value of $\zvect_1$:
\begin{flalign*}
&\begin{bmatrix}
    r_1\\
    \theta_1
\end{bmatrix}=
\begin{bmatrix}
    r_0-\eta f(\theta_0+\frac{\eta}{2}r_0)-\eta C r_0+\sqrt{2 C\eta}w\\
    \theta_0+\frac{\eta}{2}r_0+\frac{\eta}{2}\left(r_0-\eta f(\theta_0+\frac{\eta}{2}r_0)-\eta C r_0+\sqrt{2 C\eta}w\right)
\end{bmatrix}=\\
&\begin{bmatrix}
    r_0\\
    \theta_0
\end{bmatrix}+\begin{bmatrix}
    -\eta f(\theta_0)-\frac{\eta^2}{2}r_0 \frac{\partial f}{\partial \theta}+\mathcal{O}(\eta^3)-\eta C r_0+\sqrt{2 C\eta}w\\
    \frac{\eta}{2}r_0+\frac{\eta}{2}\left(r_0-\eta f(\theta_0)-\eta C r_0+\sqrt{2 C\eta}w\right)+\mathcal{O}(\eta^3)
\end{bmatrix}=\\
&\begin{bmatrix}
    r_0\\
    \theta_0
\end{bmatrix}+\begin{bmatrix}
    \eta^{\frac{1}{2}}\sqrt{2 C}w+\eta \left(-f(\theta_0)-C r_0\right)+\eta^2(-\frac{1}{2}r_0 \frac{\partial f}{\partial \theta}) \\
    \eta r_0+\frac{\eta^{\frac{3}{2}}}{2}\sqrt{2 C}w+\eta^2\left(-\frac{1}{2} f(\theta_0)-\frac{1}{2} C r_0\right)
\end{bmatrix}+\mathcal{O}(\eta^3)=\\
&\begin{bmatrix}
    r_0\\
    \theta_0
\end{bmatrix}+\begin{bmatrix}
    \delta_r\\
    \delta_\theta
\end{bmatrix}+\mathcal{O}(\eta^3).
\end{flalign*}

Consequently, dropping the dependence on $\zvect_0$ (whenever unambiguous), 
\begin{flalign*}
&\phi(\zvect_1)=\phi+\p_r \phi \delta_r+\p_\theta \phi \delta_\theta+\frac{\p_{rr}\phi}{2}\delta_r^2+\frac{\p_{\theta\theta}\phi}{2}\delta_\theta^2+\p_{r\theta}\phi \delta_r\delta_\theta+\frac{\p_{rrr}\phi}{6}\delta_r^3+\frac{\p_{\theta\theta\theta}\phi}{6}\delta_\theta^3+\\
&\frac{3\p_{rr\theta}\phi}{6}\delta_r^2\delta_\theta+\frac{3\p_{\theta\theta r}\phi}{6}\delta_\theta^2\delta_r+\frac{\p_{rrrr}\phi}{24}\delta_r^4+\mathcal{O}(\eta^3).
\end{flalign*}

To derive the operator $\mathcal{U}$ we need to take the expected value of both sides. We need the following equalities, that with an abuse of notation are valid up to $\mathcal{O}(\eta^3)$
\begin{flalign*}
&\E(\delta_r)=-\eta f-\frac{\eta^2}{2}r\p_\theta f-\eta C r \\
&\E(\delta_\theta)=\eta r-\frac{\eta^2}{2} f-\frac{\eta^2}{2} C r\\
&\E(\delta_r^2)=\eta^2C^2r^2+\eta^2f^2+2\eta^2Cpf+2\eta C\\
&\E(\delta_\theta^2)=\eta^2r^2\\
&\E(\delta_r\delta_\theta)=\eta^2 C+\eta^2(-fr-Cr^2)\\
&\E(\delta_r^3)=\eta^2 6C \left(-f-C r\right)\\
&\E(\delta_\theta^3)=0\\
&\E(\delta_r^2\delta_\theta)=\eta^2 2Cr\\
&\E(\delta_\theta^2\delta_r)=0\\
&\E(\delta_r^4)=\eta^2 12 C^2
\end{flalign*}
By expanding the operator $\mathcal{U}$ in powers of $\eta$ we then obtain
\begin{flalign}\label{expu}
&\mathcal{U}=\E(\phi(z_1))=\phi+\eta\underbrace{\left(\left(\p_r\phi\right)(-f-Cr)+\left(\p_\theta\phi\right) r+\left(\p_{rr}\phi\right) C\right)}_{\mathcal{L}}+\frac{\eta^2}{2}( \underbrace{-\left(\p_r\phi\right) r\p_\theta f}_{B} \underbrace{-\left(\p_\theta\phi\right)f}_{F}\underbrace{-\left(\p_\theta\phi\right)Cr}_{J}\nonumber\\
&\underbrace{+\left(\p_{rr}\phi\right)C^2r^2}_{K}\underbrace{+\left(\p_{rr}\phi\right)f^2}_{G}\underbrace{+\left(\p_{rr}\phi\right)2Crf}_{H}+\underbrace{\left(\p_{\theta\theta}\phi\right)r^2}_{A}\underbrace{-2fr\left(\p_{r\theta}\phi\right)}_{C}\underbrace{-2Cr^2\left(\p_{r\theta}\phi\right)}_{D}\underbrace{+2C\left(\p_{r\theta}\phi\right)}_{M}\nonumber\\
&\underbrace{-2Cf\left(\p_{rrr}\phi\right)}_{I}\underbrace{-2C^2r\left(\p_{rrr}\phi\right)}_{L}\underbrace{+\left(\p_{rr\theta}\phi\right)2Cr}_{E}\underbrace{+\left(\p_{rrrr}\phi\right)C^2}_{N})+\mathcal{O}(\eta^3).
\end{flalign}

The operator of interest is $\mathcal{L}=r\p_\theta-f\p_r-Cr\p_r+C\p_{rr}$.
Expanding instead
\begin{flalign}\label{expl}
&\mathcal{L}^2=(r\p_\theta-f\p_r-Cr\p_r+C\p_{rr})^2=\nonumber\\
&r\p_\theta(r\p_\theta-f\p_r-Cr\p_r+C\p_{rr})+\nonumber\\
&-f\p_r(r\p_\theta-f\p_r-Cr\p_r+C\p_{rr})+\nonumber\\
&-Cr\p_r(r\p_\theta-f\p_r-Cr\p_r+C\p_{rr})+\nonumber\\
&C\p_{rr}(r\p_\theta-f\p_r-Cr\p_r+C\p_{rr})=\nonumber\\
&\underbrace{r^2\p_{\theta\theta}}_{A}\underbrace{-r\p_\theta f\p_r}_{B}\underbrace{-rf\p_{r\theta}}_{C}\underbrace{-Cr^2\p_{r\theta}}_{D}\underbrace{+Cr\p_{rr\theta}}_{E}+\nonumber\\
&\underbrace{-f\p_\theta}_{F}\underbrace{-fr\p_{r\theta}}_{C}\underbrace{+f^2\p_{rr}}_{G}+fC\p_r\underbrace{+fCr\p_{rr}}_{H}\underbrace{-fC\p_{rrr}}_{I}+\nonumber\\
&\underbrace{-Cr\p_\theta}_{J}\underbrace{-Cr^2\p_{r\theta}}_{D}\underbrace{+fCr\p_{rr}}_{H}+C^2r\p_r\underbrace{+C^2r^2\p_{rr}}_{K}\underbrace{-C^2r\p_{rrr}}_{L}+\nonumber\\
&\underbrace{2C\p_{r\theta}}_{M}\underbrace{+Cr\p_{rr\theta}}_{E}\underbrace{-fC\p_{rrr}}_{I}-2C^2\p_{rr}\underbrace{-C^2r\p_{rrr}}_{L}\underbrace{+C^2\p_{rrrr}}_{N}
\end{flalign}
we see that not all the terms match the $\eta^2$ terms of the Taylor expansions of $\mathcal{U}$. As anticipated, it is not possible to state anything quantitatively precise, but noticing that many of the summands coincide provides an hint about the \leapfrog performance.

As a side note, we stress moreover that the \leapfrog scheme can be instead easily modified to be order-two at no additional computational cost, by leveraging the results of \cref{ousol} and considering substituting the Euler step of \cref{eumom} with the analytical one. %This would be similar in spirit to the scheme discussed in \cite{chen2015convergence}, where however {\color{red}(unnecessary?)} splittings are considered.
